# Supplementary material for: How to Quantify Polarization in Models of Opinion Dynamics
Source: arXiv:2110.11981 source file (2021-10-26)
Supplement: Supplementary file 1 [file appendix.tex]

% !TeX root = main.tex
\appendix 
\section{Variance reduction over time}
\label{app:var_decrease}

Prove variance monotonically decreases.
